# Supplementary material for: Panoptica -- instance-wise evaluation of 3D semantic and instance segmentation maps
Source: arXiv:2312.02608 source file (2023-12-05)
Supplement: Supplementary file 1 [file appendix.tex]

\clearpage
\setcounter{section}{41}
\section{Appendix}
\input{body/appendix/benchmark}
