# Supplementary material for: Panoptica -- instance-wise evaluation of 3D semantic and instance segmentation maps
Source: arXiv:2312.02608 source file (2023-12-05)
Supplement: Supplementary file 2 [file tab_perf_test.tex]

\begin{table*}[htbp!]
    \centering
    \begin{tabularx}{\textwidth}{lcccccc}
        \toprule
        \multicolumn{3}{c}{Test Sample} & Machine & \multicolumn{3}{c}{Time Measurements (sec)}                                                                               \\
        \cmidrule(lr){1-3}
        \cmidrule(lr){4-4}
        \cmidrule(lr){5-7}
        Type & Foreground Size & Number of Instances &  & Inst. Approx. & Inst. Matching & Evaluation \\
        \midrule
        T2w Spine & $(170, 512, 17)$ & s & Work machine & $0.019 \pm 0.002$ & $0.416 \pm  0.023$ & $5.024 \pm 0.036$\\
    \end{tabularx}
    \caption{
        Performance test of the \textit{panoptica} package.
        Each test report the mean and standard deviations across 50 iterations.
        All measurements are given in seconds.
        The sample size are the number of pixels in each dimension, while foreground size gives the actual size of segmented areas in the input dimensions.
        The input sample size is cropped down to the foreground size.
        While instance approximation and instance matching are quite fast, the evaluation can take a couple of seconds, depending on the input sizes.
        As \textit{panoptica} allows the user to specify which metrics should be calculated, these times can still be individually lower.
    }
    \label{tab:perf_test}
\end{table*}

[TODO extend with more samples, different machines!]
